# Supplementary material for: Calliope-Net: Automatic Generation of Graph Data Facts via Annotated Node-link Diagrams
Source: arXiv:2308.06441 source file (2023-08-12)
Supplement: Supplementary file 1 [file 10-appendix.tex]

\section*{Appendix A}

\subsection*{Topological Graph Partition Algorithm}
\label{appendix:partition}
% Besides the graph partition strategies we introduced in Sec.~\ref{sec:graph fact generation}, 
\name can partition the selected subgraph into communities based on various topological methods as follows:
\begin{itemize}
    \item \textbf{Connected components.} \name partitions graph into a set of connected components which are not connected with each other. For every two nodes within a component, there exists at least a path connecting them.
    \item \textbf{Greedy modularity community.} Clauset-Newman-Moore greedy modularity maximization method~\cite{clauset2004finding} obtains communities from graph by greedily combining community pairs to increase modularity most.
    % \item \textbf{Fluid communities.} Fluid Communities~\cite{pares2017fluid} is a propagation-based community detection algorithm which requires the users to assign the number of communities. We implement it on the largest connected component of $G^{\prime}$ and assign the number of communities as $10$.
    % \item \textbf{Girvan–Newman algorithm.} Classic Girvan–Newman algorithm~\cite{girvan2002community} detects communities from $G^{\prime}$ by repeatedly removing the edges with the highest betweenness centrality.
\end{itemize}

\subsection*{Topological Feature}
\label{appendix:feature}
For the features calculated, besides the aggregation of node attributes, \name can explore a wide range of topological features. For the topological features of the node, the candidate features are:
\begin{itemize}
    \item \textbf{Degree.} Degree of a node denotes the number of edges connecting to the node.
    \item \textbf{PageRank score.} PageRank~\cite{page1999pagerank} score measures the importance of a node in terms of the network topology. The damping parameter is set as $\alpha=0.85$.
    \item \textbf{Eigenvector centrality.} Eigenvector centrality~\cite{bonacich1987power} of every node is obtained based on the corresponding entry of the eigenvector for the largest eigenvalue.
\end{itemize}

For topological features of the community, the options are:
\begin{itemize}
    \item \textbf{Count.} The count refers to the \# of nodes in the community.
    \item \textbf{Inside edge number.} This feature measures the total number of edges within a community.
    \item \textbf{Density.} The density of a community is defined as $\frac{2\times\texttt{Inside edge number}}{\texttt{Count}\times(\texttt{Count}-1)}$.
    \item \textbf{Average degree.} The average degree of a community is defined as $\frac{2\times\texttt{Inside edge number}}{\texttt{Count}}$.
    \item \textbf{Triangle Participation Ratio.} The triangle participation ratio is defined as the ratio of nodes which belong to at least one triangle. 
    \item \textbf{Cut ratio.} The cut ratio~\cite{fortunato2010community} is defined by the ratio of observed cut over all the possible cuts.
    \item \textbf{Conductance.} The conductance~\cite{shi2000normalized} refers to the ratio of observed cut over the total edge volume of a community.
    \item \textbf{Maximum-out degree fraction.} The out degree fraction (ODF) refers to the fraction of edges of a node (in a community) that point out of the community. Thus, the maximum-ODF~\cite{flake2000efficient} refers to the maximum of ODFs of all the nodes in the community.
    \item \textbf{Average-out degree fraction.} Average-ODF~\cite{flake2000efficient} refers to the average value of ODFs of all the nodes in the community.
    \item \textbf{Separability.} Separability~\cite{shi2000normalized} refers to the ratio of the number of the internal edges over the number of the external edges.
\end{itemize}

\subsection*{Interestingness Score}
\label{appendix:interestingness}
% Given the calculated features $\{\rho(G^{\prime}_i)\}$ from previous steps, 
The goal of interestingness score is to evaluate whether this observed feature vector is significantly common or not for a fact type-specific assumption. 
% For example, given a bibliography network, the feature vector extracted by setting $\phi:\textrm{Domain=Visualization}$, $\psi:\textrm{Node}$, $\rho:\textrm{Degree}$ represents the degree distribution of researchers in the visualization domain. A common assumption about the degree distribution is that it should follow the power law distribution. Hence, if the observed feature vector is significantly different from the power law distribution, it will be evaluated as interesting from the \emph{distribution} perspective. 
The technique has been well-studied by existing automatic insight extraction arts~\cite{ding2019quickinsights,tang2017extracting,wang2019datashot,shi2020calliope}. We follow part of their designs and evaluate the interestingness from the following perspectives.
% The common solution for evaluating interestingness in automatic insight extraction arts~\cite{ding2019quickinsights,tang2017extracting,wang2019datashot} is to define a fact type-specific null hypothesis and use the $1-\textrm{p-value}$ as the interestingness metric.
\begin{itemize}
    \item \textbf{Extreme.} The null hypothesis of \emph{Extreme} fact type is that (1) the feature vector in descending order should follow the power law distribution and (2) the regression residuals should follow the Gaussian distribution. The specific procedure is as follows.
    \begin{itemize}
        \item Sort the feature vector in descending order.
        \item Remove the maximum value $x_{\texttt{max}}$ and use the remaining values to fit a power law distribution with $\beta=0.7$.
        \item Infer a Gaussian distribution $D$ based on the residuals of power law regression.
        \item Predict the maximum value $\tilde{x}_{\texttt{max}}$ with the residual $R$ as $|\tilde{x}_{\texttt{max}}-x_{\texttt{max}}|$.
        \item The $p$-value is equivalent to $p(R|D)$ and the interestingness is 1-$p$.
    \end{itemize}
    For the \emph{Extreme} fact type, the focus is the corresponding community/node of the maximum feature value.
    
    \item \textbf{Evenness.} The evenness fact type is to determine if the entries from the feature vector are uniformly distributed. The null hypothesis of \emph{Evenness} fact type is that the feature vector should be the a constant vector (i.e., all the entries fall into one value which is non-uniform). Hence, the specific procedure is as follows.
    \begin{itemize}
        \item Perform the Chi-squared test against the null hypothesis to obtain the $p$-value.
        \item The interestingness is 1-$p$.
    \end{itemize}
    For the \emph{Evenness} fact type, no focus is provided for visualization.
    
    \item \textbf{Distribution.} The distribution fact type is to determine if entries of the feature vector are well-modeled by a Gaussian distribution. Hence, the null hypothesis of \emph{Distribution} fact type is that the feature vector comes from a Gaussian distribution. The specific procedure is as follows.
    \begin{itemize}
        \item Perform the Shapiro–Wilk test on the given feature vector to obtain the $p$-value.
        \item The interestingness is 1-$p$.
    \end{itemize}
    For the \emph{Distribution} fact type, no focus is provided for visualization.
    
    \item \textbf{Proportion.} The more dominant the leading value is in the feature vector, the more interesting \name evaluates it as. This interestingness evaluation requires the feature vector to be non-negative. Hence, the specific procedure is as follows.
    \begin{itemize}
        \item Sort the feature vector in descending order and obtain the maximum value $x_{\texttt{max}}$. 
        \item Calculate the proportion of the leading value $\frac{x_{\texttt{max}}}{\sum x}$
        \item The interestingness is $\min{(1, \frac{2\times x_{\texttt{max}}}{\sum x})}$.
    \end{itemize}
    For the \emph{Proportion} fact type, the focus is the corresponding community/node of the maximum feature value.
    
    \item \textbf{Rank.} The \emph{Rank} fact type shares the similar null hypothesis with the \emph{Extreme} fact type but focus on top-$k$ values from the feature vector. In our settings, we set $k=3$. The specific procedure is as follows.
    \begin{itemize}
        \item Sort the feature vector in descending order.
        \item Remove the largest values $x_{\texttt{max}}$ and use the remaining values to fit a power law distribution.
        \item Infer a Gaussian distribution $D$ based on the residuals of power law regression.
        \item Predict the largest value $\tilde{x}_{\texttt{max}}$ with the residual $R$.
        \item The $p$-value is equivalent to $p(R|D)$ and the interestingness is 1-$p$.
    \end{itemize}
    For the \emph{Rank} fact type, the focus is the corresponding communities/nodes of the largest three feature values.
    
    \item \textbf{Outlier.} The \emph{Outlier} fact type is designed for the node-level feature vector. Intuitively, if the feature value of a node is significantly different from the average feature value of its neighbors, the node tends to be labelled as an outlier. The specific procedure for detecting the outlier is as follows.
    \begin{itemize}
        \item For the $i$-th node, calculate the expected feature value $\tilde{x}_i$ by averaging the feature values of its neighbors.
        \item The outlier score of every node is the normalized difference between the expected and observed feature value as $\frac{|\tilde{x}_i-x_i|}{\max(\tilde{x}_i,x_i)}$.
        \item  The interestingness of a node is the corresponding outlier score.
    \end{itemize}
    For the \emph{Outlier} fact type, the focus is the corresponding node of the largest outlier score.
\end{itemize}

\subsection*{Measurements in Natural Language Descriptions}
The detailed descriptions for measurements are shown in Table \ref{tab:description}.

\begin{table*}[bp]

\linespread{1.5}
\setlength\aboverulesep{0pt}
\setlength\belowrulesep{0pt}
\centering
\caption{Descriptions Of Technical Terms}
\begin{tabular}{|p{0.22 \textwidth}|p{0.22 \textwidth}|p{0.4 \textwidth}|}
\toprule
\textbf{Measure}         & \textbf{Description}      & \textbf{Example}                    \\ \hline
Degree      & Super connector                    &  Node A is a super connector as it has the most connections.
\\ \hline
PageRank score         & 
Important
& 
Node A is an important node because it has 
has many connections and important neighbors.
\\ \hline
Eigenvector centrality   & 
Influential
& 
Node A is an influential node while considering 
both direct and indirect connections.
\\ \hline
Inside edge number   & 
Close internal relationship
& 
Community A has a close internal relationship based on the highest inside connections.
\\ \hline

Average degree/ Density 
& 
Highly connected 
& 
Community A is a highly connected community based on frequent internal connections.			
			
\\ \hline
Average out degree fraction/Maximum out degree fraction
& 
Strong external connectivity
& 
Community A has strong external connectivity based on frequent external connections.				
				
\\ \hline
Separability
& 
Isolated
& 
Community A is an isolated community based on scarce external connections.	
\\ \bottomrule
\end{tabular}
\label{tab:description}
\end{table*}

\vspace{5mm}

\section*{Appendix B}
\vspace{3mm}
\subsection*{Topic Skeleton Selection Algorithm}
\vspace{-3mm}
\begin{algorithm}[ht]
\SetAlgoLined
\KwIn{Topic skeleton list, $\Gamma_s = \{\gamma_1, \gamma_2,... ,\gamma_N\}$}
\KwOut{Optimal topic skeleton, $\gamma^*$}
    \While{$sum(\arrt) < limit$}{
    $\arrt := zeros(len(\Gamma_s))$\;
    $\arre := zeros(len(\Gamma_s))$\;
    \For{\texttt{$i:=0, i < len(\Gamma_s), i++ $}}{
        $\arrv[i]: = \arre[i] + \sqrt{\frac{ln (sum(\arrt))}{\arrt[i]}}$\;
    }
    
    $i':= argmax(\arrv)$\;
    $\gamma' := \Gamma[i']$\;
    $r := explore(\gamma')$\;
    $expectations[i'] = \frac{\arre[i'] * \arrt[i'] + r}{\arrt [i'] + 1}$\;
    $\arrt[i'] = \arrt [i'] + 1$\;
    }
    $i^* := argmax({\arre})$\;
    $\gamma^* := \Gamma_s[i^*]$\;
    \Return $\gamma^*$\;
    \caption{Topic Skeleton Selection} 
    \label{algo:topic}  
\end{algorithm}
\vspace{-3mm}

\subsection*{Narrative Expansion Algorithm}

Narrative expansion algorithm iteratively runs until no facts can be added to increase the objective function. As Algorithm \ref{algo:expansion} shows, the algorithm receives a topic skeleton $S$ and adds the suitable facts to form complete narratives. 
The algorithm starts by constructing the candidate set of the initial topic tree by $initializeCandidates$ function. The valid candidates include all the facts which are related to the facts already in the current topic tree in terms of the logical relation or topological relation mentioned before.
Then the function runs a \textit{while} iteration to choose the next relation to add.
% searching all the candidate relations of the initial skeleton. 
% The algorithm calculates the gain by the rewards function $rewards$.
In each iteration, the algorithm enumerates the candidates and evaluate the candidate relation $r$ by objective function $f$ when $r$ is added to the topic tree by function $addRelation$ to form a new topic skeleton $S'$
% when the relation $r$ is added to the story $S$. The reward is evaluated based on function $reward$. Then
After enumerating the candidate set, the algorithm can specify the relation $r_{next}$ who has the largest objective function and add it to the topic tree by $addRelation$.
% In each iteration, the algorithm search the best-fit candidate relation $r_{next}$ which has the largest rewards and add it to the topic tree by $addLink$ function. 
Then, the algorithm will update the candidate set by three steps.
% The updating progress comprises of three steps.
% After each iteration, the algorithm update the candidate set based on the newly added relation $r_{next}$. 
First, the algorithm updates the old candidate set $X_{old}$ by removing the relations who share the same successor fact with the newly added relation $r_{next}$.
Then, the algorithm generates the new candidate set $X_{new}$ by selecting the facts related with the relation $r_{next}$ and not in the current skeleton $S$.
% It gets all the related facts with their corresponding relations by function $getRelatedFacts$. Then the candidate set removes all the relations whose successor fact is the newly added in that the topic tree structure does not allow any loop. 
Finally, the algorithm merges the original and new candidate set to obtain the candidate to use in the next iteration.
The algorithm stops and outputs the topic tree if the $r_{next}$ is null, which means no fact can increase the total gain, the algorithm stops and outputs the result.

\begin{algorithm}[!ht]
\SetAlgoLined
\KwIn {Topic Skeleton, $S_{in}$}
\KwOut {Complete Structure, $S_{out}$}
$X := initializeCandidates(S)$\;
$S := S_{in}$\;
\While{True}{
    $g_{max} := 0$\;
    $r_{next} := null$\;
      \For{\texttt{r in X}}{
        $S' := addRelation(S, r)$\;
        $g := f(S') - f(S)$\;
         \If{ $g > g_{max}$}{
              $g_{max} := g$\;
              $r_{next} := r$\;
          }
      }
       
        % \State \texttt{<do stuff>}
      \If{ $r_{next} = null$}{
              break\;
      }
    $S := addRelation(S, r_{next})$\;
    $X_{old} := X.filter(r=>r.f_s \neq r_{next}.f_s)$\;
    $X_{new} := getRelatedFacts(r_{next}.f_s)$\;
    $X_{new} := X_{new}.filter(r=>r.f_s \not\in S.facts)$\;
    $X := merge(X_{new}, X_{old})$\;
}
%   instructions\;
%   \eIf{condition}{
%   instructions1\;
%   instructions2\;
%   }{
%   instructions3\;
%   }
$S_{out} := S$\;
\Return $S_{out}$\;
\caption{Narrative Expansion Algorithm}
\label{algo:expansion}
\end{algorithm}
